# Supplementary material for: An aperiodic monotile
Source: arXiv:2303.10798 ancillary file (2024-07-03)
Supplement: Supplementary file 1 [file neighbours.pdf]

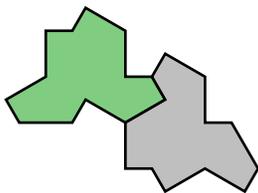

<-1,-1,8,1,0,-4>

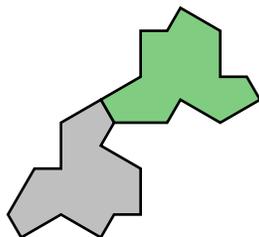

<0,1,0,1,0,-6>

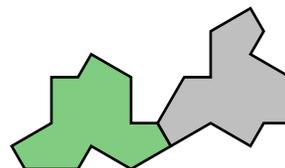

<0,1,6,1,0,0>

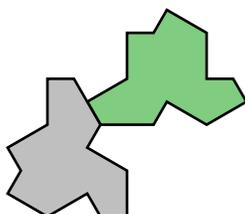

<1,0,-2,-1,-1,-2>

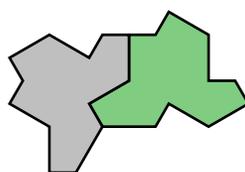

<0,-1,-2,1,1,-2>

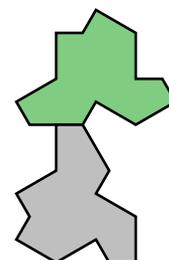

<1,0,2,-1,-1,-4>

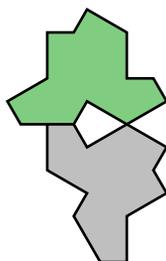

<-1,0,6,1,1,-6>

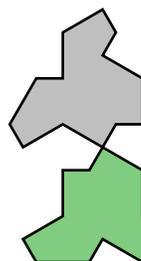

<0,1,-2,1,0,4>

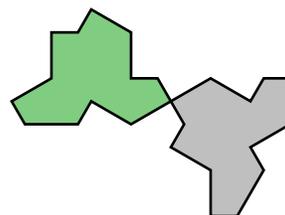

<0,-1,8,1,1,-4>

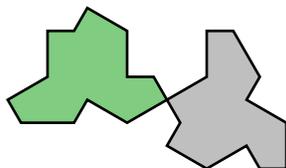

<1,0,6,-1,-1,0>

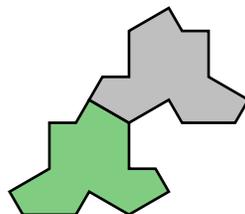

<-1,-1,4,0,1,4>

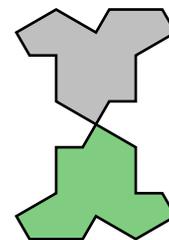

<-1,0,0,0,-1,6>

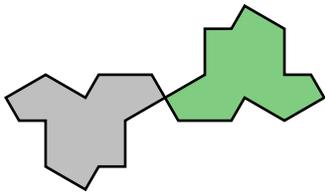

<-1,0,-2,0,-1,-2>

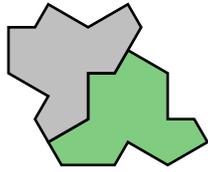

<0,-1,-2,-1,0,4>

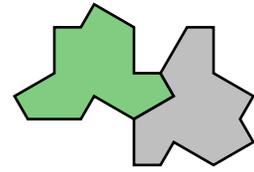

<0,1,6,-1,-1,0>

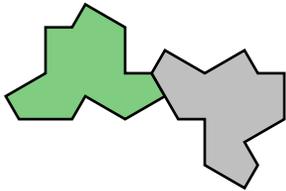

<1,1,6,-1,0,0>

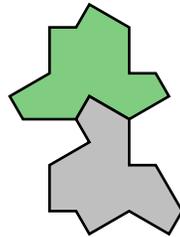

<-1,-1,6,1,0,-6>

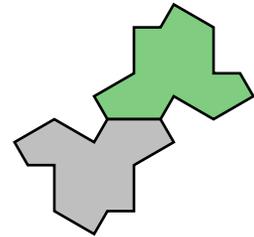

<-1,0,2,0,-1,-4>

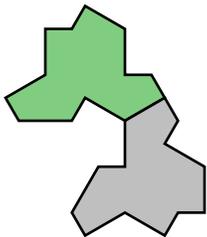

<0,1,6,1,0,-6>

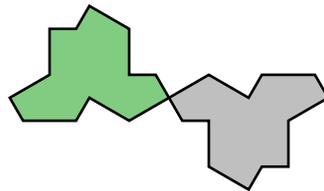

<-1,0,10,0,-1,-2>

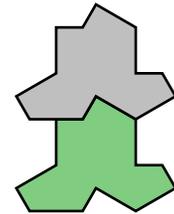

<1,0,-2,0,1,4>

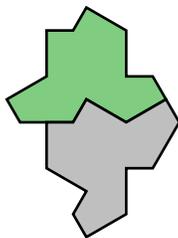

<0,-1,4,-1,0,-2>

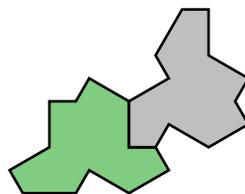

<0,1,4,-1,-1,4>

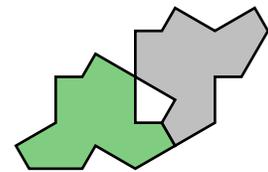

<0,-1,4,-1,0,4>

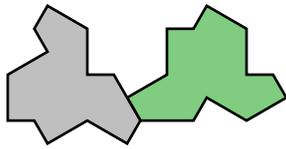

<-1,-1,-2,1,0,-2>

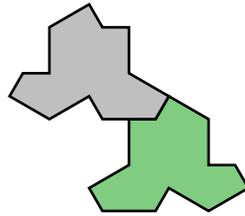

<-1,-1,-2,0,1,4>

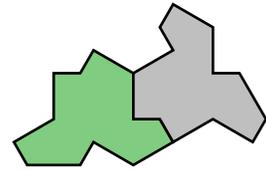

<-1,-1,6,1,0,0>

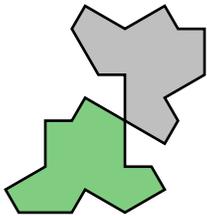

<1,1,0,-1,0,6>

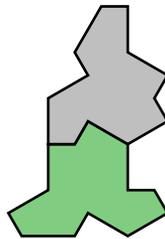

<0,1,0,-1,-1,6>

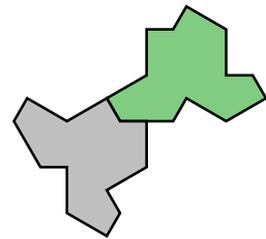

<1,1,-2,-1,0,-2>

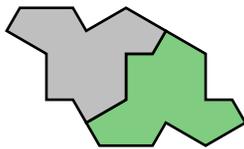

<1,1,-4,0,-1,2>

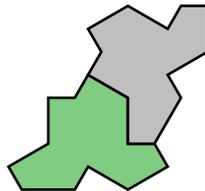

<0,-1,2,1,1,2>

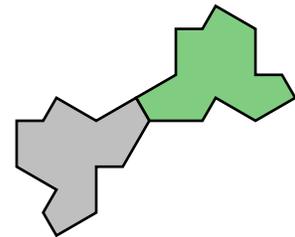

<0,-1,-2,-1,0,-2>

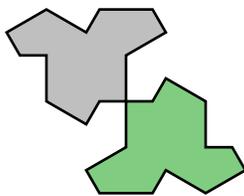

<-1,0,-2,0,-1,4>

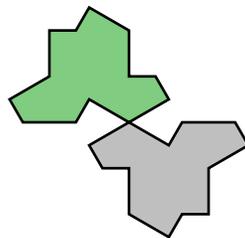

<-1,0,8,0,-1,-4>

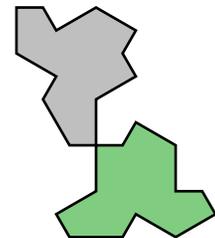

<-1,0,-2,1,1,4>

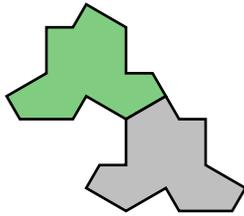

<-1,-1,8,0,1,-4>

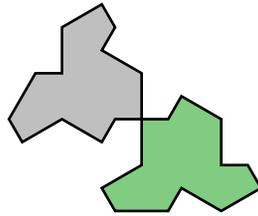

<0,1,-4,1,0,2>

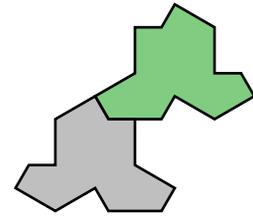

<-1,-1,2,0,1,-4>

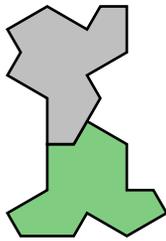

<0,-1,-2,1,1,4>

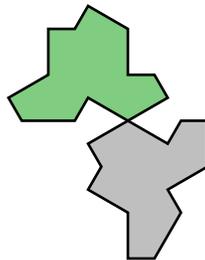

<0,-1,6,1,1,-6>

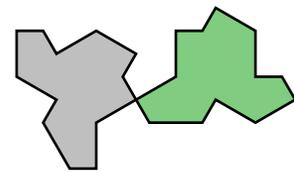

<-1,0,-2,1,1,-2>

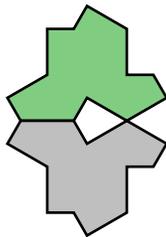

<1,1,2,0,-1,-4>

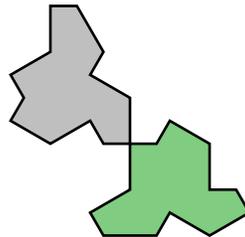

<1,0,-6,-1,-1,6>

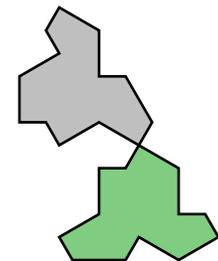

<-1,-1,-2,1,0,4>

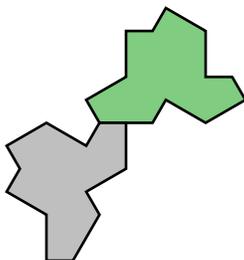

<0,-1,0,1,1,-6>

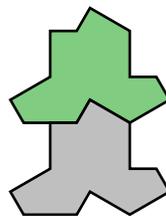

<1,0,2,0,1,-4>

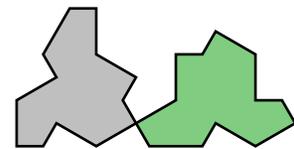

<0,1,-4,-1,-1,2>

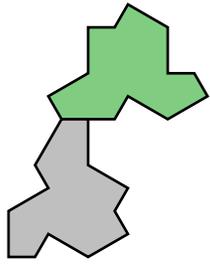

<0,1,2,-1,-1,-4>

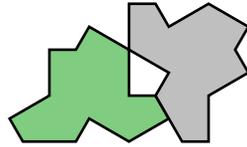

<-1,0,6,1,1,0>

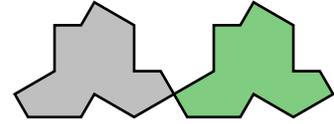

<1,0,-6,0,1,0>

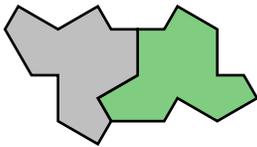

<1,1,-4,-1,0,2>

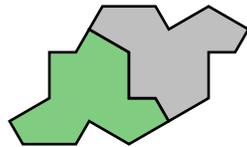

<1,1,2,0,-1,2>

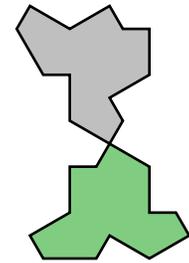

<1,1,-4,-1,0,8>

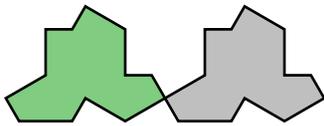

<1,0,6,0,1,0>

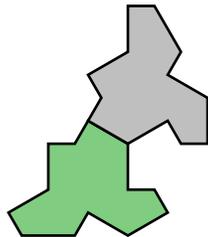

<1,0,0,-1,-1,6>

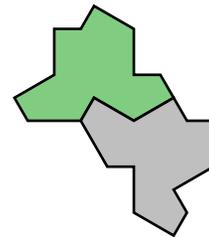

<1,1,4,-1,0,-2>

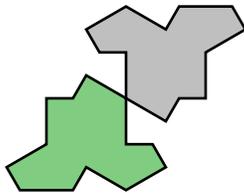

<-1,0,4,0,-1,4>
